# Supplementary material for: Dexterous Imitation Made Easy: A Learning-Based Framework for Efficient Dexterous Manipulation
Source: arXiv:2203.13251 source file (2022-03-24)
Supplement: Supplementary file 1 [file appendix.tex]

\section{Appendix}
